# Supplementary material for: STATE: A Robust ATE Estimator of Heavy-Tailed Metrics for Variance Reduction in Online Controlled Experiments
Source: arXiv:2407.16337 source file (2024-07-23)
Supplement: Supplementary file 1 [file appendix.tex]

% \section{Appendix}
% \appendix
% \section{Appendix: Supplementary experimental results}
